# Supplementary material for: What are the visual features underlying human versus machine vision?
Source: arXiv:1701.02704 source file (2017-11-07)
Supplement: Supplementary file 1 [file supplementary_v1.tex]

\begin{figure}[t]
\begin{center}
   \includegraphics[width=1\linewidth]{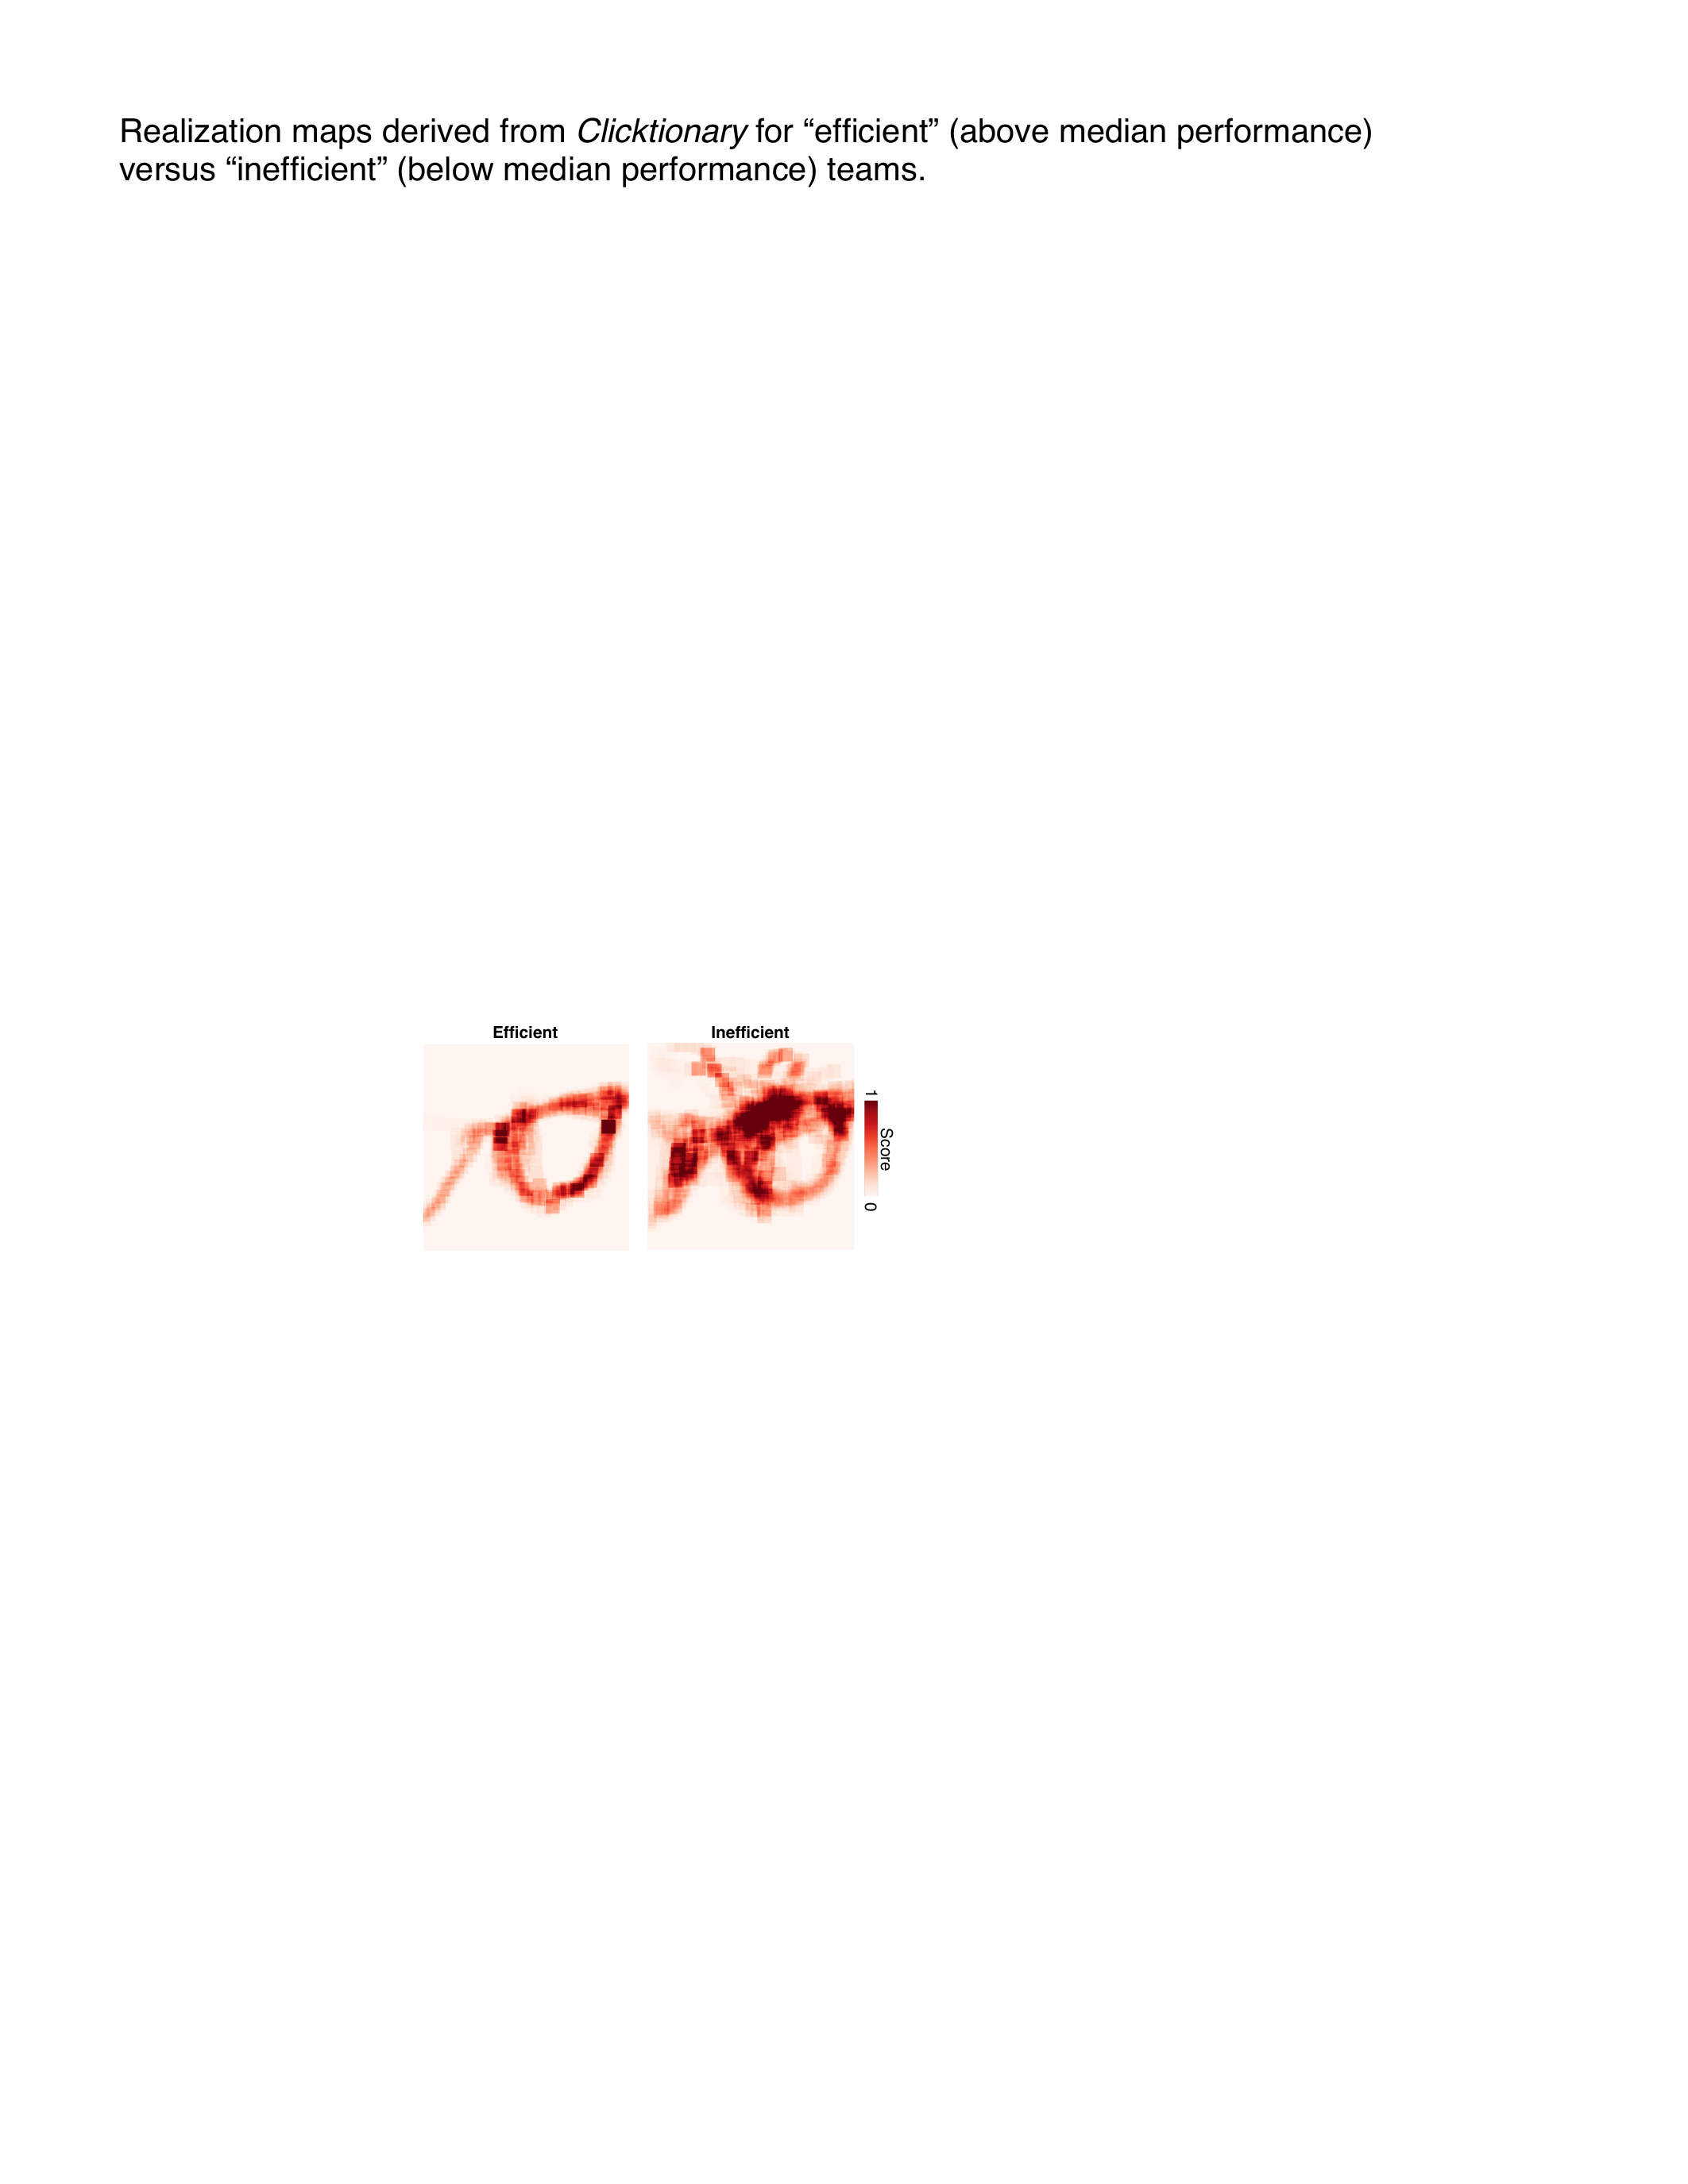}
\end{center}
   \caption{Realization map features vary according to how efficiently a participant pair recognized images. On the left, the mean realization map from pairs with above-median efficiency in recognizing glasses (i.e. faster recognition). On the right, the mean realization map from below-median pairs. The above image is representative of the typical differences between these groups.}
\vspace{}\label{split_half_viz}
\end{figure}

Despite the strong agreement we observed between \emph{Clicktionary} participants, we found that realization maps were affected by player performance. Applying a median split to the number of bubbles it took before a student in a pair recognized an image revealed two qualitatively different realization maps (Fig.~\ref{split_half_viz}). Maps from the efficient group (i.e. number of bubbles is below median split) were sparser than those from the less efficient group. More work is needed to understand if these differences indicate increased noise from the latter group or belie different sets of visual features selected by each.
%\enlargethispage{5mm}

\begin{figure}[t]
\begin{center}
   \includegraphics[width=1\linewidth]{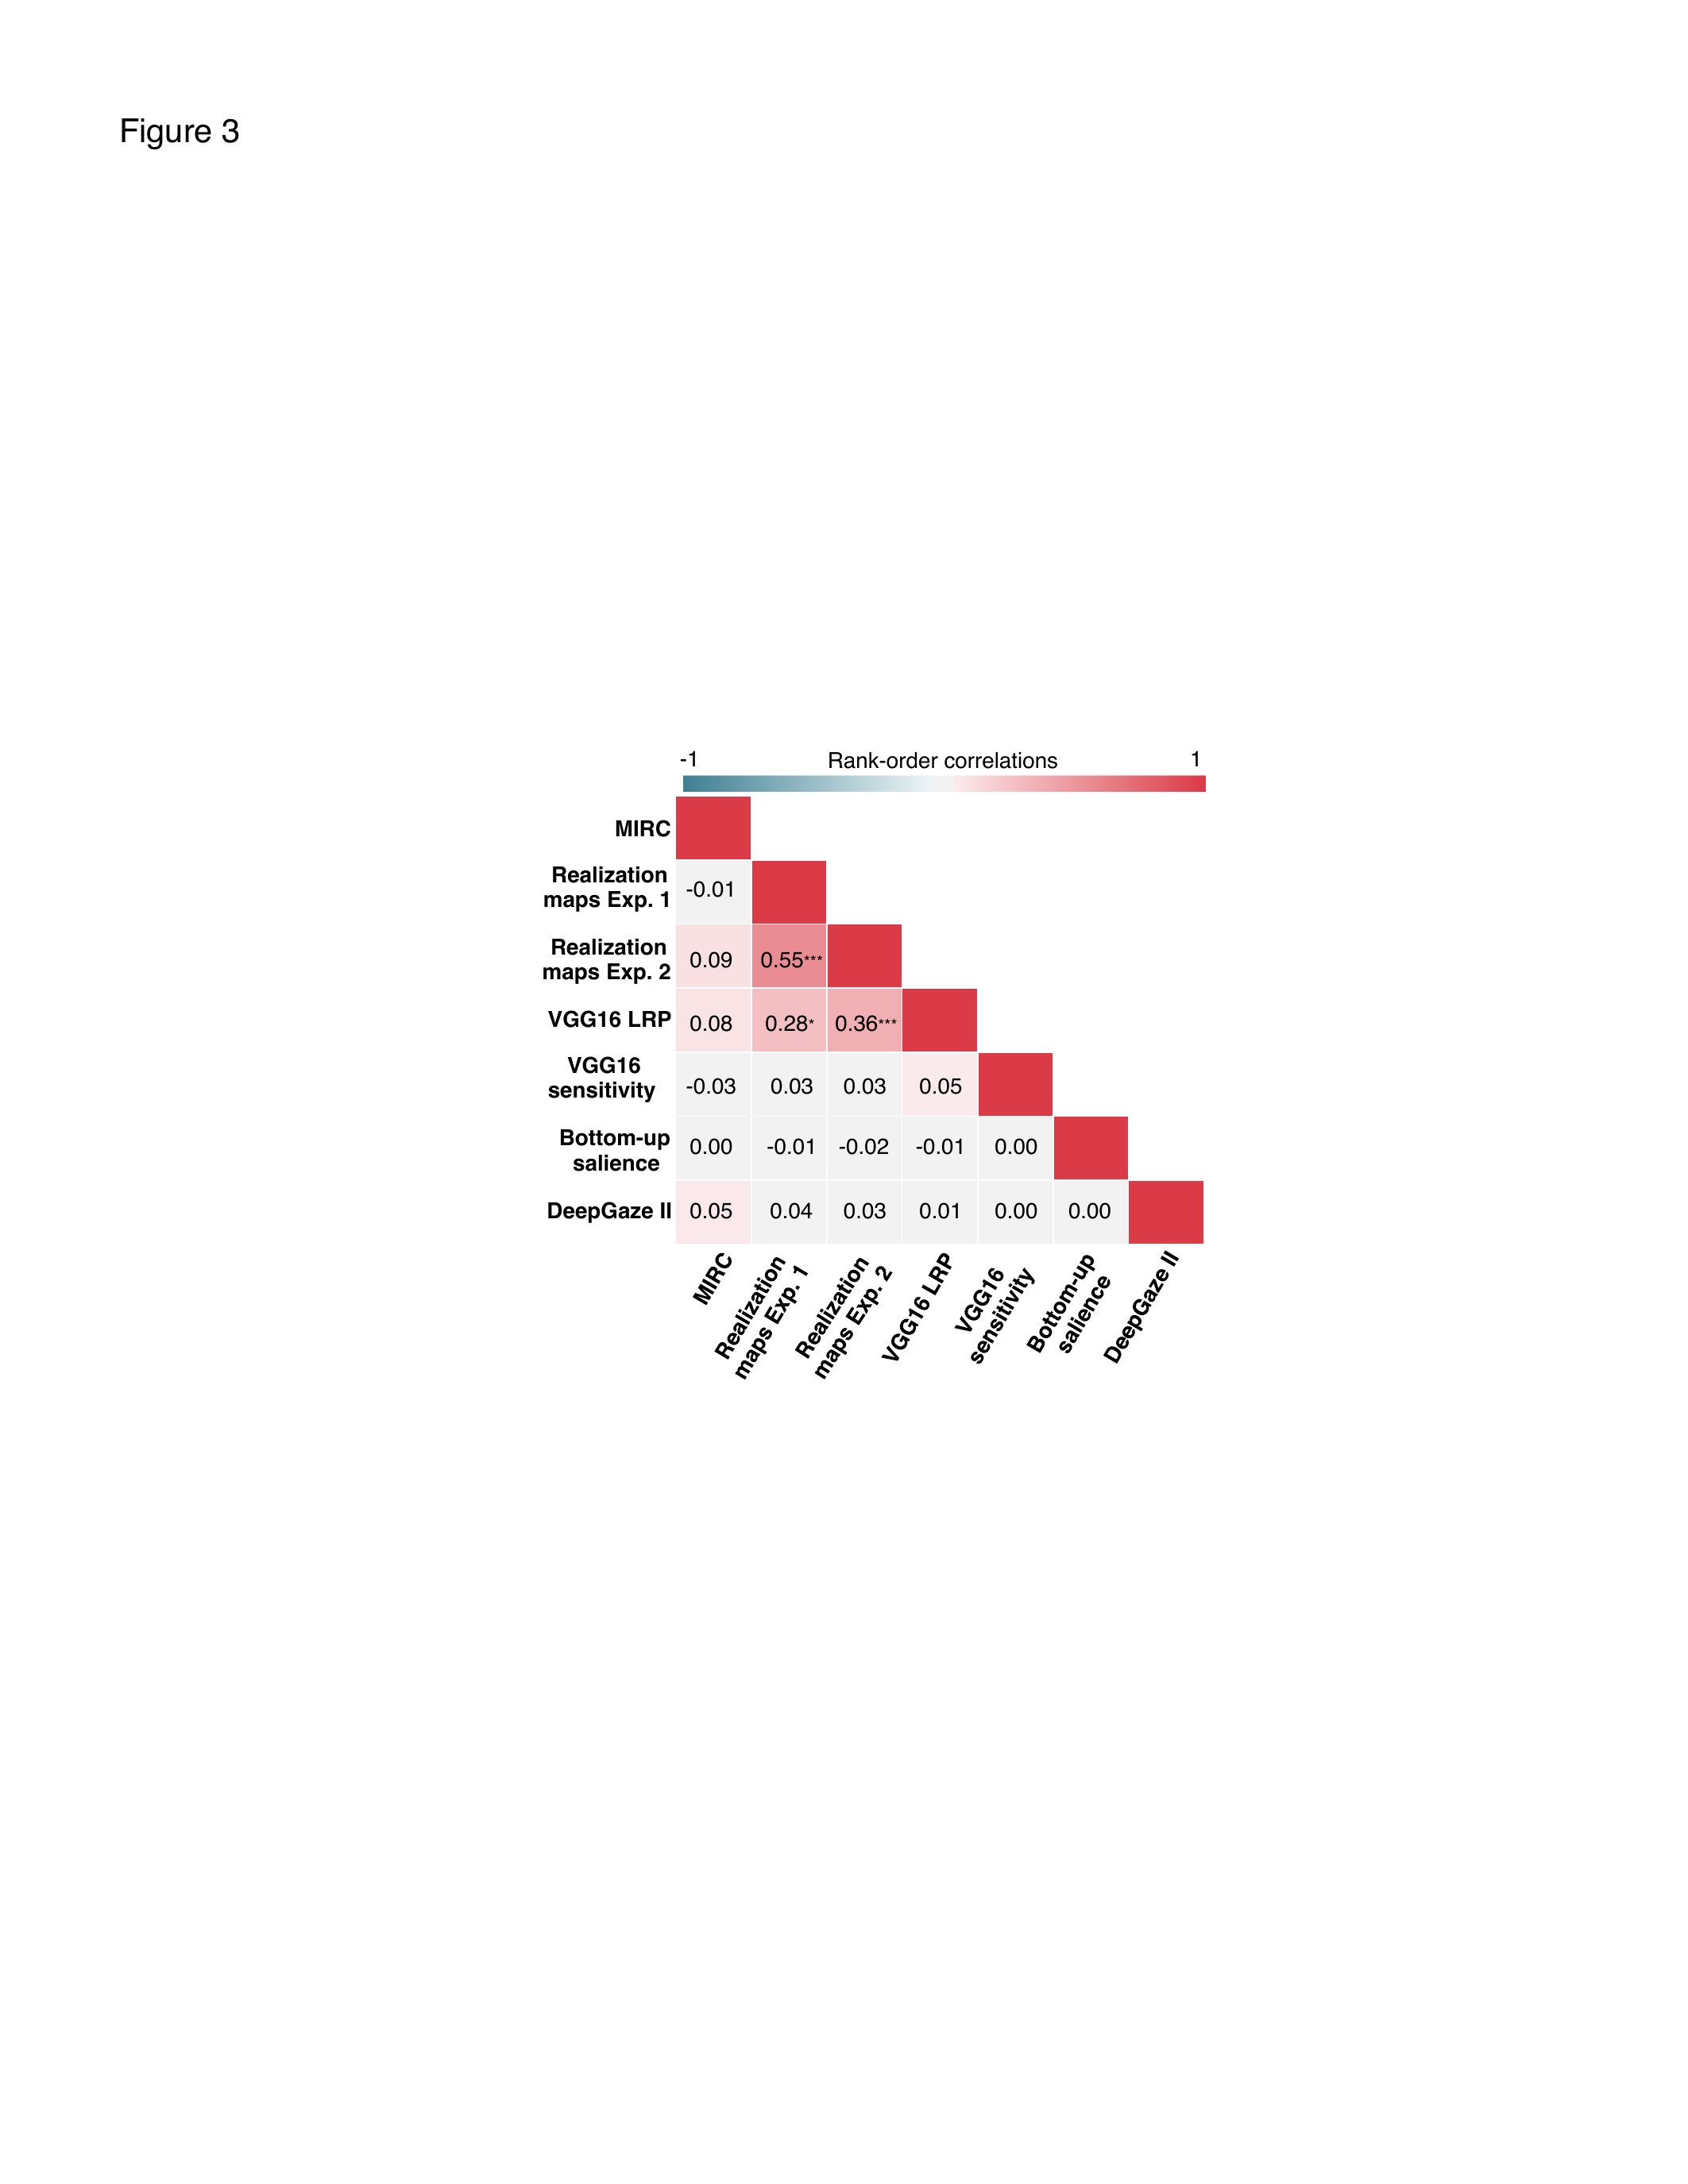}
\end{center}
   \caption{Mean pairwise correlations between realization maps derived from humans and DCNs using images from~\cite{Ullman2016-ea}. Cells are colored according to the strength and direction of association between maps.}
\vspace{}\label{fig_mirc_corr}
\end{figure}

\begin{figure}[t]
\begin{center}
   \includegraphics[width=1\linewidth]{latex_figures/figure_6}
\end{center}
   \caption{A depiction of the interface at  \url{Clickme.ai} for large-scale acquisition of realization maps, and continuous measurement of its impact on DCN performance. After a certain number of clicks are accrued, the application trains the weights of MLnet, a model for predicting eye fixations, to predict realization maps in images. These maps are incorporated into VGG16 through ''cooperative training'', that will drive it towards human perception.}
\vspace{}\label{webapp}
\end{figure}
